# Supplementary material for: BKL bounces outside homogeneity: Gowdy symmetric spacetimes
Source: arXiv:2408.12427 source file (2024-08-22)
Supplement: Supplementary file 1 [file appendix.tex]

%auto-ignore
\appendix

\section{Proof of the weighted product estimate} \label{app:weightedl2}

In Appendix~\ref{app:weightedl2} we provide a proof of the weighted $L^2$ product estimate Lemma~\ref{lem:weightedl2}. By a simple density argument, it suffices to assume that $f$ and $g$ are smooth, and for convenience we work in $L^p$--spaces with respect to the measure $w^2 dx$ i.e.~with
\begin{equation*}
    \| f \|_{L^p(w^2 dx)} = \left( \int_{\mathbb{S}^1} |f(x)|^p w^2(x) \, dx \right)^{\frac{1}{p}}
\end{equation*}

For $0 \leq k \leq K$, we shall moreover define $p_k = \frac{2K}{k}$ (where $p_0 = \infty$) and the quantities $F_k$ and $G_k$ as:
\begin{gather*}
    F_0 = \| f \|_{L^{\infty}(w^2 dx)}, \qquad F_k = \sum_{i=0}^{k-1} \| \partial_x^{k-i} f \|_{L^{p_k}(w^2 dx)} \| \partial_x W \|_{L^{\infty}(w^2 dx)}^i \text{ for } 1 \leq k \leq K, \\[0.3em]
    G_0 = \| g \|_{L^{\infty}(w^2 dx)}, \qquad G_k = \sum_{i=0}^{k-1} \| \partial_x^{k-i} f \|_{L^{p_k}(w^2 dx)} \| \partial_x W \|_{L^{\infty}(w^2 dx)}^i \text{ for } 1 \leq k \leq K.
\end{gather*}
With this notation, Lemma~\ref{lem:weightedl2} is reduced to proving that
\begin{equation} \label{eq:weightedl2_0}
    \| \partial_x^M f \, \partial_x^N g \|_{L^2(w^2 dx)} \lesssim_{M, N} F_0 G_k + G_0 F_k.
\end{equation}

In order to prove such an estimate, our first goal will be to show that for $0 \leq k \leq K$, one has
\begin{equation} \label{eq:weightedl2_interp}
    F_k \lesssim F_0^{\frac{K-k}{K}} F_K^{\frac{k}{K}}.
\end{equation}
We do this in several steps. Firstly, for $0 < k < K$ one may use the identity 
\begin{multline*}
    \partial_x (w^2 |\partial_x^k f|^{p_k - 2} \, \partial_x^k f \cdot \partial_x^{k-1} f) = w^2 |\partial_x^k f|^{p_k} 
    \\[0.2em] + w^2 (p_k-1) |\partial_x^k f|^{p_k-3} \, \partial_x^{k+1} f \cdot \partial_x^k f \cdot \partial_x^{k-1} f + 2 w^2 \partial_x W \cdot |\partial_x^k f|^{p_k-2} \partial_x^k f \cdot \partial_x^{k-1} f.
\end{multline*}

Integrating this identity over $x \in \mathbb{S}^1$, one thereby deduces that
\[
    \int_{\mathbb{S}^1} |\partial_x^k f|^{p_k} w^2 \,dx \lesssim
    \int_{\mathbb{S}^1} |\partial_x^k f|^{p_k-2} \, |\partial_x^{k+1} f| \, |\partial_x^{k-1} f| w^2 \, dx + \int_{\mathbb{S}^1} |\partial_x^k f|^{p_k - 1} \, |\partial_x^{k-1} f| \, |\partial_x W| w^2\,dx,
\]
and an application of H\"olders inequality to the two integrals on the right hand side yields (all $L^p$ spaces are with respect to the measure $w^2 dx$):
\[
    \| \partial_x^k f\|_{L^{p_k}}^{p_k} \lesssim \| \partial_x^k f \|_{L^{p_k}}^{p_k-2} \| \partial_x^{k-1} f \|_{L^{p_{k-1}}} \left( \| \partial_x^{k+1} f \|_{L^{p_{k+1}}} + \| \partial_x^k f \|_{L^{p_{k+1}}} \| \partial_x W \|_{L^{\infty}} \right).
\]
Thus by the definition of $F_k$ one concludes that
\[
    \| \partial_x^k f \|_{L^{p_k}}^2 \lesssim F_{k-1} F_{k+1}.
\]

On the other hand, a standard $L^p$ interpolation estimate (where the implied constants are importantly independent of the measure associated to the $L^p$ space), one has that for $1 \leq j \leq k - 1$,
\[
    \| \partial_x^{k-j} f \|_{L^{p_k}}^2 \| \partial_x W \|_{L^{\infty}}^{2j} \lesssim \| \partial_x^{k-j} f \|_{L^{p_{k-1}}} \| \partial_x W \|_{L^{\infty}}^{j-1} \cdot \|\partial_x^{k-j} f \|_{L^{p_{k+1}}} \| \partial_x W \|_{L^{\infty}}^{j+1} \leq F_{k-1} F_{k+1}.
\]
Combining the above two equations, one therefore has that $F_{k}^2 \lesssim F_{k-1} F_{k+1}$. 

It is straightforward to go from this to \eqref{eq:weightedl2_interp}. For instance, assuming that all the $F_j$ are nonzero the inequality $F_j^2 \lesssim F_{j-1} F_{j+1}$ implies there is some constant $C \in \R$ such that
\begin{align*}
    - \frac{K - k}{K} \log F_0 - \frac{k}{K} \log F_K + F_k 
    &= \sum_{j=1}^{K-1} \left( - \log \frac{1}{2} F_{j-1} - \frac{1}{2} \log F_{j+1} + \log F_j \right) \cdot \left( \frac{\min\{ j(K-k), (K-j)k\}}{K}\right) \\
    &\leq C,
\end{align*}
which immediately yields \eqref{eq:weightedl2_interp}.

Finally, in order to deduce \eqref{eq:weightedl2_0} from \eqref{eq:weightedl2_interp} (and the analogous inequality for the $G_k$s) we simply apply H\"older's inequality followed by \eqref{eq:weightedl2_interp}, as follows:
\[
    \| \partial^M_x f \, \partial^N_x g \|_{L^2} \leq \| \partial^M_x f \|_{L^{p_M}} \| \partial^N_x g \|_{L^{p_N}} \leq F_M G_N \leq (F_0 G_K)^{\frac{N}{K}} (F_K G_0)^{\frac{M}{K}}.
\]
The conclusion thus follows from Young's inequality. \qed
